# Supplementary material for: PASTA: Part-Aware Sketch-to-3D Shape Generation with Text-Aligned Prior
Source: arXiv:2503.12834 source file (2025-03-17)
Supplement: Supplementary file 1 [file architecture_details.tex]

\section{Architecture Details}\label{supp:section3}
To provide a deeper understanding of our proposed framework, we present additional architectural details regarding hierarchical clustering, part-wise Gaussian grouping, and vision-language model (VLM) descriptions for different object categories.

\subsection{Hierarchical Clustering in PartGCN}
Our PartGCN module operates by clustering 16 Gaussian nodes into 4 distinct groups, allowing the model to learn structured part-level representations of objects. 
This hierarchical clustering process is performed using dendrogram-based grouping, ensuring that semantically related Gaussians are aggregated together. Fig 5
illustrates this process, showing how individual nodes are iteratively merged into higher-level clusters until four representative groups emerge. This structured partitioning significantly enhances the model’s ability to capture global shape consistency while retaining fine-grained details.

\subsection{Part-wise Gaussian Grouping Across Object Categories}
To further analyze the effectiveness of PartGCN, we visualize how different object categories—chairs, airplanes, and lamps—are decomposed into their respective Gaussian components. Fig 6 presents examples of part-wise Gaussian groupings, showcasing how each object type is divided into four primary groups based on spatial and geometric similarities. 
For instance, in chairs, the groups correspond to legs, seat, backrest, and armrests, whereas in airplanes, they represent wings, fuselage, tail, and engines. The results highlight how our approach consistently learns meaningful object decompositions across diverse categories, facilitating more interpretable and structured 3D generation.

%%%%%%%%%%%%%%%%%%%%%%%%%%%%%%%%%%%%
\input{supp_figure_txt/supp_figure5}
%%%%%%%%%%%%%%%%%%%%%%%%%%%%%%%%%%%%

\subsection{Vision-Language Model (VLM) Captions and Descriptions}
Our method incorporates textual priors extracted from a pre-trained vision-language model (VLM) to enhance semantic understanding of sketches.
To illustrate the nature of these textual embeddings, Fig 7 presents example captions and descriptions generated for chair, airplane, and lamp sketches. 
These descriptions contain key structural details, such as the number of legs on a chair, the shape of an airplane’s wings, or the shape of lamp head, providing additional contextual information that improves the model’s ability to generate accurate 3D shape reconstructions. The results demonstrate that integrating text embedding significantly aids in disambiguating abstract sketches, reinforcing the importance of multimodal learning in sketch-based 3D shape generation.

By systematically leveraging hierarchical clustering, structured part decomposition, and semantic text embeddings, our approach achieves robust and interpretable 3D reconstructions, effectively bridging the gap between abstract sketches and detailed 3D representations.
